# Supplementary material for: Lightweight Attentional Feature Fusion: A New Baseline for Text-to-Video Retrieval
Source: arXiv:2112.01832 source file (2022-07-27)
Supplement: Supplementary file 1 [file 5.Supplementary.tex]

In this supplement, we provide some details that are not included in the paper due to space limit.

\section{Experiments of video description datasets}
\rebuttal{
\subsection{The original performance}
The original performance of the state-of-the-art is reported in \cref{tab:supplementary_compare_all}, bigger is better.
\input{table/Supplementary_all_result}
}

\subsection{The \emph{Med r} scores}
The \emph{Med r} scores of the state-of-the-art is reported in \cref{tab:compair_all_supp}, smaller is better. 
\input{table/Supplementary_tab6_MedR}

\section{Experiments of TRECVID AVS 2016-2020}
The infAP of 20 queries of TV20 is shown in \cref{tab:TV20_case_study}. The CLIP-FT and CLIP2Video have achieved excellent results on the video description datasets, while on the TRECIVD, the average infAP is 0.172 and 0.180, respectively, which is 21.0\% and 17.2\% lower than LAFF. We find that for the 10 queries containing action, the LAFF outperform or is equivalent to CLIP-FT and CLIP2Video. It is proved that only using the CLIP series models pre-trained on large-scale image text data sets cannot completely solve the video text retrieval problem. Features containing temporal information, such as \textit{ircsn}, \textit{c3d}, etc., are still necessary for large-scale retrieval scenarios.
% Please add the following required packages to your document preamble:
% \usepackage{multirow}
\begin{table}[thp!]
\normalsize

\centering
\caption{\textbf{Performance of LAFF, CLIP-FT and CLIP2Video on TV20.} For CLIP-FT and CLIP2Video, no color font means the difference between infAP and LAFF is no more than 0.1, red font means infAP exceeds LAFF, and blue font means infAP is lower than LAFF.}
\label{tab:TV20_case_study}
\scalebox{0.6}{
% \arrayrulecolor{red}
\setlength{\tabcolsep}{2mm}{

\begin{tabular}{@{}lccccrrr@{}}
\toprule
\textbf{Query} & \textbf{Object} & \textbf{Person} & \textbf{Action} & \textbf{Location} & \textbf{LAFF} & \textbf{CLIP-FT} & \textbf{CLIP2Video} \\ \midrule 
641 showing an aerial view of   buildings near water in the daytime & \checkmark &  &  & \checkmark & 0.234 & 0.297 & 0.240 \\
642  a person paddling   kayak in the water & \checkmark & \checkmark & \checkmark & \checkmark & 0.430 & 0.399 & 0.445 \\
643  people dancing or   singing while wearing costumes outdoors &  & \checkmark & \checkmark &  & 0.134 & 0.080 & 0.071 \\
644  sailboats in the   water & \checkmark &  &  & \checkmark & 0.352 & {\color[HTML]{FF4343} 0.649} & {\color[HTML]{FF4343} 0.643} \\
645  a person wearing a   necklace & \checkmark & \checkmark &  &  & 0.034 & 0.036 & 0.088 \\
646  a woman sitting on   the floor & \checkmark & \checkmark &  &  & 0.163 & 0.091 & 0.106 \\
647  people or cars   moving on a dirt road & \checkmark & \checkmark & \checkmark &  & 0.267 & 0.199 & 0.223 \\
648  a man in blue jeans   outdoors & \checkmark & \checkmark &  & \checkmark & 0.053 & 0.018 & 0.081 \\
649  someone jumping   while snowboarding &  & \checkmark & \checkmark &  & 0.785 & {\color[HTML]{21A0FF} 0.448} & {\color[HTML]{21A0FF} 0.451} \\
650  one or more people   drinking wine &  & \checkmark & \checkmark &  & 0.096 & 0.054 & 0.040 \\
651  one or more people   skydiving &  & \checkmark & \checkmark &  & 0.489 & {\color[HTML]{21A0FF} 0.352} & 0.427 \\
652  a little boy smiling &  & \checkmark & \checkmark &  & 0.165 & 0.197 & 0.203 \\
653  group of people   clapping &  & \checkmark & \checkmark &  & 0.349 & {\color[HTML]{21A0FF} 0.082} & {\color[HTML]{21A0FF} 0.120} \\
654  one or more persons   exercising in a gym &  & \checkmark & \checkmark & \checkmark & 0.253 & 0.227 & 0.179 \\
655  one or more persons   standing in a body of water &  & \checkmark & \checkmark & \checkmark & 0.023 & 0.018 & 0.031 \\
656  a long haired man & \checkmark & \checkmark &  &  & 0.400 & {\color[HTML]{21A0FF} 0.277} & {\color[HTML]{21A0FF} 0.217} \\
657  a woman with short   hair indoors & \checkmark & \checkmark &  & \checkmark & 0.020 & 0.061 & 0.054 \\
658  two or more people   under a tree & \checkmark & \checkmark &  & \checkmark & 0.034 & 0.035 & 0.058 \\
659  a church from the   inside & \checkmark &  &  & \checkmark & 0.342 & {\color[HTML]{21A0FF} 0.188} & 0.255 \\
660  train tracks during   the daytime & \checkmark &  &  &  & 0.524 & {\color[HTML]{21A0FF} 0.361} & {\color[HTML]{21A0FF} 0.211} \\ \bottomrule
\end{tabular}

}
}

\end{table}
